# Supplementary material for: SentiNet: Detecting Localized Universal Attacks Against Deep Learning Systems
Source: arXiv:1812.00292 source file (2020-05-09)
Supplement: Supplementary file 1 [file appendix.tex]

\section{Using a Faster-RCNN with \tool{}}

As Faster-RCNN is an object detection network, we paid particular attention when connecting it to \tool{}. First, the prediction of Faster-RCNN consists of bounding boxes, classes and confidence of the detected objects. Instead of processing these outputs, we bypass the bounding box prediction layer and connect \tool{} directly to the class likelihood output. In doing so, \tool{} will have access to classes and confidence values only. Second, the Faster-RCNN network detects objects that are often a small part of the background scene, in contrast to cropped images often used for classification tasks. To modify our input to be compatible with the detection network as a classification task, we take the image we intend to classify and place it onto a larger image. As an example, with an image of dimension $h \times W$, we can create a larger blank image of $H \times W$ where $H = h \times n$ and $W = w \times n$, with a carefully chosen n value.  We then place our image at the coordinates $h, w$, and input as our ROI proposal $bbox = (h, w, 2h, 2w)$ as our starting x, starting y, ending x, and ending y coordinates. This larger image is projected into a feature map using spatial pyramid techniques before we feed it through the network with our ground-truth bounding box ($bbox$) as the ROI input. This technique allows us to leave unchanged the performance of the Faster-RCNN.
